# Supplementary material for: Observing the onset of outflow collimation in a massive protostar
Source: arXiv:1507.05285 source file (2015-07-19)
Supplement: Supplementary file 1 [file SupMat_carrasco-gonzalez_etal_astroph.pdf]

# Supporting Online Material

## Materials and Methods

### A. Observations and data processing

We observed W75N(B) with the Karl G. Jansky Very Large Array (VLA) of the National Radio Astronomy Observatory (NRAO) in its A-configuration at C (6 cm), U (2 cm), K (1.3 cm), and Q (7 mm) bands. Total continuum bandwidths were 4, 6, 7.8, and 8 GHz at C, U, K, and Q bands, respectively. Simultaneously to the continuum, we also observed the $5_1 - 6_0A^+$ $CH_3OH$ maser transition (rest frequency = 6.6685192 GHz; C band), and the $6_{16} - 5_{23}$ $H_2O$ maser transition (rest frequency = 22.235080 GHz; K band) with narrow bandwidths of 4 and 8 MHz, respectively. A summary of the observation setups is shown in table S1.

Complex gain calibration was made by observing J2007+4029. Flux and bandpass calibration were achieved with observations of the standard flux calibrator 3C286. We used resolved models (available in Common Astronomy Software Applications [CASA]; version 4.1.0; *30*) at all bands for this flux calibrator. The phase center of our observations towards W75N(B) was $\alpha$(J2000)=$20^h38^m36.485^s$, $\delta$(J2000)=$+42°37'34.19''$. A first calibration of the data was performed with CASA using the VLA Calibration Pipeline provided by the NRAO (version 1.2.0; *31*). Then, after inspection of the calibrated data, we performed additional data editing and re-run the pipeline when needed. Finally, self-calibration of the continuum emission was performed for each band. In the case of the K band continuum, after an initial calibration, we used a strong $H_2O$ maser (∼3,600 Jy) observed simultaneously in the narrow spectral line bandwidth of 8 MHz to self-calibrate its emission, and then applying the obtained phase and amplitude corrections to the continuum data.

Deconvolved images for each band were obtained with the task *clean* of CASA using the multi-scale multi-frequency deconvolution algorithm described in (*32*). We explored several values of the parameter *robust* for weighting the uv data, to optimize the signal-to-noise ratio and angular resolution in our studies. We detected radio continuum emission at all four bands towards VLA 1, VLA 2, VLA 3 (Fig. 1) and also towards four additional sources located $\gtrsim 2''$ away from these three sources. On the other hand, we also detected water maser emission towards VLA 1 and VLA 2. Methanol masers are mostly detected towards VLA 1, with the exception of three weak masers (∼40 mJy, $V_{LSR}$ ∼12.5 km $s^{-1}$) detected ∼$0.3''$ southwest from VLA 2 (∼390 au at the source distance of 1.3 kpc). In this paper, we concentrate on the results obtained towards the source VLA 2. The observational results on the other sources detected in the W75N(B) region will be presented and discussed elsewhere.

## B. Spatial alignment of the different continuum bands

To improve the accuracy in the relative position of the water masers detected at K band with respect to the continuum emission at the other different bands, images shown in Figs. 1 and 2 were aligned by assuming that the position of source VLA 3 is the same at all bands. We choose VLA 3 for the alignment because it is the brightest source in the field, its observed morphology does not change with the different continuum bands and angular resolutions, and its intensity distribution is nearly Gaussian. Therefore, we modified the astrometry of the C, U, and Q band images in a way that the absolute position of VLA 3 is the same as in the self-calibrated K band continuum image. The applied spatial shifts were $\lesssim$ 30 mas in all cases. We emphasize that the astrometry of the K band continuum image was not changed, and thus it is still very accurately aligned with the water masers. From the signal-to-noise ratio (SNR) of the K band continuum emission of VLA 2, we estimate that the $1\sigma$ accuracy in the relative positions between the water masers and the continuum (plotted in Figs. 1 and 2) is better than $\sim$1 mas [obtained from beam/(2$\times$SNR); (*33*)]. For the methanol masers plotted in Figs. 1 and 2, we estimate an accuracy of $\sim$30 mas in their relative positions with respect to the K band continuum image (the maximum spatial shift we applied to align the different continuum bands of our VLA observations).

## C. K band continuum in VLA 2 as observed in epochs 1996 and 2014

From the K band data obtained in 1996 (*10*) and 2014 (this paper), we imaged the continuum emission from VLA 2 with natural weight of visibilities, to optimize the sensitivity, and with the same restoring circular beam of $0.12''$ (Fig. 2). In table S2 we give the image parameters for both epochs, such as the intensity peak, total flux density, source size (obtained from elliptical Gaussian fits), as well as the rms of the images. The resulting values for the source size in 1996, and the fact that the peak intensity is similar to the flux density, indicate that VLA 2 is undistinguishable from a point source in that epoch. However, in 2014 the core of the radio continuum emission is elongated in the northeast-southwest direction, with its FWHM major axis being clearly resolved. This elongation is also clearly seen in the image obtained with the uv data uniformly weighted (Fig. S2). Fitting the source size in the uv plane for both epochs (assuming the visibilities corresponding to an elliptical disk) gives results consistent with those of the image fits.

In addition to the elongated structure observed in the core of the K band continuum emission in 2014, we detected weak extended emission at distances $\lesssim 0.3''$ ($\lesssim$390 au) southwest of its peak position (Figs. 1, 2, S2). This emission is at levels of $\sim$40-100 $\mu$Jy beam$^{-1}$ ($\sim$4-10 times the rms of the image obtained with natural weighting, $\sim$10 $\mu$Jy beam$^{-1}$). This weak extended emission was not detected in 1996 (*10*). Given that the sensitivity of the K band continuum data in 1996 data was $\sim$150 $\mu$Jy beam$^{-1}$ (a factor of $\sim$15 lower than in

2014; see Fig. S3), it is possible that this weak emission was already present in 1996, but not detected.

Ideally, a more direct comparison between the radio continuum data in both epochs could be obtained by obtaining maps with a similar frequency and uv coverage. However this was not possible in our case, since the frequencies observed in 1996 were not covered in the 2014 observations. Moreover, the observing time in both epochs were very different (7 hours in 1996 vs 45 min in 2014), which implies a much poorer uv coverage and lower sensitivity in the 2014 data if the bandwidths in both epochs are matched. In fact, by selecting a 25 MHz window, we obtain a sensitivity of $\sim$190 $\mu$Jy beam$^{-1}$, not enough for a clear detection of VLA 2 (peak $\sim$700 $\mu$Jy beam$^{-1}$, epoch 2014).

There are several arguments favoring that our radio continuum observations show the evolution from a point source (1996) to an extended elongated source (2014): *i)* The core of the continuum emission traced at FWHM has a resolved size in 2014 (Figs. 1, 2, S2; table S2); *ii)* the intensity peak has decreased from 1.42$\pm$0.15 mJy beam$^{-1}$ (1996) to 0.82$\pm$0.01 mJy beam$^{-1}$ (2014), while the total flux density maintains similar values in both epochs, 1.69$\pm$0.25 mJy (1996) and 1.33$\pm$0.03 mJy (2014) (table S2). This suggests that the continuum emission in 2014 arises from a larger region than in 1996, as traced by the weak elongated structure seen in 2014 (Figs. 1, 2, S2); *iii)* the water masers in 1996 are distributed on an almost round shell around the continuum emission, while in 2014 they show an elliptical structure around the elongated radio continuum emission (Fig. 2). We have followed the evolution of the water maser shell through very long baseline interferometry (VLBI) observations during the last 13 years (1999-2012). We found that the shell has evolved from an almost circular shell of $\sim$142 mas ($\sim$185 au) diameter expanding in multiple directions, to an elliptical structure of $\sim$272$\times$146 mas ($\sim$354$\times$190 au) oriented northeast-southwest, mainly expanding in that direction (see Fig. S1; [*14*]).

**D. Spectral energy distribution of VLA 2**

To study the dependence of the radio continuum emission of VLA 2 with frequency, we made additional cleaned maps by dividing each of the different U, K, and Q bands in chunks of 1 GHz bandwidth. In table S3 and Fig. S4 we give the corresponding values of the flux density ($S_\nu$) and the size of the major axis of the VLA 2 source ($\theta$) as function of frequency ($\nu$). We have not extended this procedure to the C band continuum given that the beam size at this frequency is $\sim$0.3$''$ does not allow us to separate the emission of VLA 2 from that of VLA 3 (see Fig. 1).

The spectral energy distribution (SED) in the U, K, and Q bands can be fitted by two components. One is dominated by free-free emission with a spectral index $\alpha \simeq 0.61\pm0.04$

($S_\nu \propto \nu^\alpha$) in the lower frequency bands (U and K). At the highest frequencies (Q band) the emission deviates in ∼30% (∼0.5 mJy) from this behavior, showing a steeper spectral index that can be explained with the presence of thermal dust emission with $\alpha_{dust} \simeq 3.5\pm0.5$ (Fig. S4). If we take into account an upper limit to the continuum emission at 217 GHz (*20*), the spectral index of the dust emission seems to be near to 3.

From the thermal dust emission at 44 GHz (∼0.5 mJy after subtracting the free-free emission), we made a rough estimate for the total (dust + gas) mass of $\gtrsim$ 0.001 $M_\odot$. To obtain this value, we assumed optically thin emission, constant dust temperature $T_d$ = 300 K (which is a reasonable value for the gas temperature at distances of tens of au from the massive protostar), gas-to-dust mass ratio = 100, and dust opacity coefficient $\kappa$(44 GHz) $\lesssim$ 0.2 cm$^2$ g$^{-1}$ (from [*23*] and adopting a dust opacity index $\beta_{\rm dust} \gtrsim 1$). This calculated mass has large uncertainties (up to two orders of magnitude), mainly due to the unknown temperature structure, dust-to-gas mass ratio, and grain size distribution around VLA 2 (strongly affecting $\kappa$; see [*34,35*]). Observational data at higher frequencies, with enough angular resolution (better than ∼0.5″) to isolate VLA 2 from the other protostars in the region (VLA 1 and VLA 3), would help to obtain a more accurate SED to properly model the thermal dust component (*34,35*).

## E. Toroidal environmental density stratification model

What our new VLA observations show is that the radio continuum emission from W75N(B)-VLA 2 has evolved in ∼18 yr from a compact source (1996) to an elongated one (2014) with physical characteristics of a thermal, collimated ionized wind oriented northeast-southwest (Figs. 1, 2, S2; see discussion in the main text of this paper). This evolution is consistent with that of the associated expanding water maser shell, which, in a similar time-span, has also evolved from an almost circular shell expanding in multiple directions, to an elliptical structure mainly expanding in the northeast-southwest direction (Fig. S1; [*14*]). We interpret all these results in terms of a massive protostar ejecting an episodic, short-lived uncollimated wind, that is shock-exciting the masers, and is expanding within a toroidal environmental density stratification, as discussed below.

The interaction of a wind with the surrounding environment produces a two-shock structure that travels away from the star. The outer shock accelerates the environment, while the inner shock decelerates the wind. For young stars with moderate wind velocities (few hundred of km s$^{-1}$), both the inner and outer shocks are, in general, radiative and results in the formation of a thin expanding shell bounded by the two shocks. (*36*) developed a general method for solving problems of wind-driven shells moving into a medium with an arbitrary density distribution, and an arbitrary time dependence of the wind. We apply this method to the case of an steady isotropic wind surrounded by a torus of dense material.

The parameters of the wind are its mass-loss rate ($\dot{M}_w$) and its terminal velocity ($V_w$). For the toroidal environmental density distribution, we assume a function of the form

$$\rho(R,\theta) = \frac{\rho_0}{1+\left[\frac{R}{R_c(\theta)}\right]^2}\,, \tag{1}$$

where R is the distance from the star, $R_c(\theta)$ is the latitude-dependent radial size of the core given by

$$R_c(\theta) = R_0(1+p\sin^2\theta)\,, \tag{2}$$

where $\theta$ is the polar angle, measured from the symmetry axis of the torus, and $R_0$ is a constant. In eq. (E1), $\rho_0$ represents the density of the core, while in eq. (E2), $p$ is related to the density contrast between the equator ($\theta=\pi/2$) and the pole ($\theta=0$) of the toroidal environment. From these equations we see that for $R \ll R_c$ the density is nearly uniform, that is, independent of direction and radial size, while for $R \gg R_c$, the density decreases as $1/R^2$, which is the behavior of the density of self-gravitating isothermal spheres at large distances.

A straightforward application of the method developed by (*36*) gives the radial size of the shell $R_s(\theta,t)$ as a function of direction and time in an implicit form,

$$t = t_i + \frac{t_0}{R_0}R_s + \xi^{\frac{1}{2}}\left(\frac{R_c}{R_0}\right)^2 t_0\sqrt{\left(\frac{R_s}{R_c}\right)^2 - 2\left(\frac{R_s}{R_c}\right)\arctan\left(\frac{R_s}{R_c}\right) + ln\left[1+\left(\frac{R_s}{R_c}\right)^2\right]}\,, \tag{3}$$

where

$$t_0 = \frac{R_0}{V_w}\,, \tag{4}$$

and

$$\xi = 4\pi R_0^2\rho_0\left(\frac{V_w}{\dot{M}_w}\right)\,. \tag{5}$$

Thus, the model has five parameters: $t_i$, $R_0$, $t_0$ (or $V_w$), $\xi$, and $p$. From eq. (E3), for $R \ll R_c$ (times close to $t_i$), we find

$$t \simeq t_i + \frac{R_s}{V_w} + \frac{\xi^{\frac{1}{2}}}{\sqrt{6}}\frac{R_s^2}{R_0 V_w}\,, \tag{6}$$

with the corresponding shell velocity

$$V_s = \frac{dR_s}{dt} = V_w\left[1-\left(\frac{2}{3}\xi\right)^{\frac{1}{2}}\frac{R_s}{R_0}\right]\,. \tag{7}$$

Eqs. (E6) and (E7) show several important physical characteristics of the initial expansion of the shell at small radii: *i)* the shell grows isotropically (with no angular dependence);

*ii)* the initial velocity of the shell is the velocity of the wind; and *iii)* the shell decelerates, and this is due to the incorporation of environmental material with zero velocity.

On the other hand, the dynamical behavior of the shell at large distances from the star can also be found from eq. (E3) for $R \gg R_c$. The result for the radial size is

$$t \simeq t_i - \frac{\pi}{2}\xi^{\frac{1}{2}}\frac{R_c^2}{R_0 V_w} + \left(1 + \xi^{\frac{1}{2}}\frac{R_c}{R_0}\right)\left(\frac{R_s}{V_w}\right) , \tag{8}$$

and for the velocity

$$V_s = \frac{V_w}{1 + \xi^{\frac{1}{2}}\frac{R_c}{R_0}} \tag{9}$$

The expansion at large radii has two important physical characteristics: *i)* there is a strong angular dependence of the shell growth velocity, and thus of its radial size, much larger along the symmetry axis of the torus than along its equator; *ii)* the velocity of the shell tends, asymptotically, to an angular dependent constant value. We thus expect the shell to become elongated in the direction of the symmetry axis of the torus (see representation of the model in Fig. 3). The constancy of the shell velocity at large distances is due to the fact that, in this limit, the momentum rate injected into the shell by the wind exactly equals the momentum rate needed to accelerate the swept-up environment (at rest) to the velocity of the shell.

We have highlighted above some of the dynamical properties of the shocked shell in the isotropic-wind/torus model. Let us now apply this model to the expanding shell of water masers observed in W75N(B)-VLA 2. It is clear that the model can explain, in principle, the most important characteristic of the expanding shell of masers: the transition from an uncollimated, nearly spherical outflow into a collimated, elongated outflow in a short period of time since the shell expands faster along the symmetry axis of the surrounding torus (Fig. 3).

To estimate the values of the five parameters of our model for the case of the expanding shell of VLA 2, we used the sizes of the semi-major and semi-minor axis of the water maser shell for four epochs between 1999.25 and 2014.54, reported in (*14*) (see also Fig. S1). We identify these axes (major and minor) with the direction along the symmetry axis of the surrounding torus ($\theta = 0$) and along the equator ($\theta = \pi/2$), respectively.

In our estimates we did not consider the 2005.89 epoch, since the behavior of the semi-major axis of the ellipse reported for this epoch cannot be explained within the framework of our model (its value in this epoch is greater than that in the next epoch). In the fitting procedure, we fix the values for $p$ and $V_w$, and then performed a least-square fitting to the data varying the remaining parameters ($\xi$, $R_0$, and $t_i$). Our main results are:

1) The values of $t_i$ and $R_0$ are nearly insensitive to the exact values of $p$ and $V_w$ (provided $p \gtrsim 5$), and well restricted:

$$t_i = 1983 - 1985 \text{ (year of ejection)}; \;\; R_0 = 19 - 23 \text{ mas } (25 - 30 \text{ au})$$

2) The values of $\xi$ are also insensitive to the value of $p \gtrsim 5$, but strongly depend on $V_w$, in a nearly quadratic form.

As an example, we show in table S4 the values of the fitted parameters for $p = 100$ and several values of $V_w$. Clearly, to further restrict the values of $V_w$ and thus $\xi$, we need to set some further constraints. One of them can be provided by the radio continuum observations. We have shown that the radio continuum emission of VLA 2 arises from an ionized wind that also drives the maser shell, since it has the frequency and size dependence predicted by theory, $\sim\nu^{0.61}$ and $\sim\nu^{-0.7}$, respectively [*(37,38)*; Fig. S4]. Using the observed flux density of 1 mJy at $\nu = 20$ GHz (table S3), in the model of *(37)*, we find a constraint to the parameters of a fully ionized wind,

$$\left(\frac{\dot{M}_w}{10^{-7}\ M_\odot\ yr^{-1}}\right) \simeq 3.2 \left(\frac{V_w}{100\ km\ s^{-1}}\right) . \tag{10}$$

As an additional constraint, we follow *(39)* by requiring that the ram pressure of the shock onto the dense environment has to be in the range $P \simeq (0.3\text{-}0.4)\times10^{-5}$ dyn cm$^{-2}$, in order to provide the appropriate density and temperature in the cooling region of the shock for pumping water maser emission at 22 GHz. From this constraint, we obtain a condition for the pre-shock density,

$$\rho_s = \frac{P}{V_s^2} , \tag{11}$$

where $V_s$ is shock velocity. The pre-shock density and the density of the core ($\rho_0$) are related by eq. (E1) if we take $R$ as the radial size of the shell $R_s$. Let us consider the direction along the symmetry axis of the torus ($\theta = 0$), then $R_c = R_0$. Assuming, further that $R_s \gg R_0$, it follows from eq. (E1) that

$$\rho_0 R_0^2 \simeq \rho_s R_s^2 . \tag{12}$$

We can now substitute eqs. (E11) and (E12) in (E5) to obtain,

$$\xi = 4\pi \left(\frac{R_s}{V_s}\right)^2 \left(\frac{V_w}{\dot{M}_w}\right) P . \tag{13}$$

Numerically,

$$\xi \simeq 445 \left(\frac{P}{10^{-5}\ dyn\ cm^{-2}}\right) \left[\frac{(R_s/100\ au)}{(V_s/10\ km\ s^{-1})}\right]^2 \left[\frac{(V_w/100\ km\ s^{-1})}{(\dot{M}_w/10^{-7}\ M_\odot\ yr^{-1})}\right] . \tag{14}$$

We take $R_s$ = 136 mas (177 au; the semi-major axis of the fitted water maser shell in epoch 2012.54) and $V_s = 30$ km s$^{-1}$ (the outward velocity of the maser shell as estimated by [*14*]). The ratio between the wind velocity and the wind mass loss rate is given by eq. (E10). We then have,

$$\xi \simeq 49 \left( \frac{P}{10^{-5}\ \mathrm{dyn\ cm^{-2}}} \right) .$$

Using this result, together with the range of possible values for the ram pressure of the shock wave, $P \simeq$ (0.3-0.4)$\times10^{-5}$ dyn cm$^{-2}$, we find the range of possible values for the parameter $\xi \simeq$ 15-200, allowing us to find constraints for the following parameters: $V_w \simeq$ 110-350 km s$^{-1}$, $R_0 \simeq$ 20-22 mas (26-29 au), $t_i \simeq$1983.8-1985.0 (from table S4), $n_0 \simeq$ (4-6)$\times10^7$ cm$^{-3}$ (from eq. E5), and $\dot{M}_w \simeq$ (4-11)$\times10^{-7}$ M$_\odot$ yr$^{-1}$ (from Eq. E10).

The model assumes that the torus is seen almost edge-on. This is consistent with the observations by Surcis et al. (2014), who in VLA 2 derive an angle between the magnetic field and the line-of-sight of $+84^{\circ}{}^{+6^{\circ}}_{-10^{\circ}}$, which means that the magnetic field is almost on the plane of the sky.

## F. Predictions of radio recombination lines

The detection of radio recombination lines (RRLs) from VLA 2 would be very important, since they could be used to directly measure the ionized wind velocity. However, these lines are expected to be very weak, and in fact, there is no detections of thermal RRLs in ionized winds from protostars (*40*). The only reported RRL emission from an ionized wind in a massive protostar was found in Cepheus A HW2, but it seems to be a non-thermal maser line (*41*).

The expected intensity of thermal RRLs ($S_L$) can be estimated from the radio continuum emission ($S_C$), following the formulation given by (*40*):

$$\frac{S_L}{S_C} = 0.19 \Big(\frac{\nu_L}{\mathrm{GHz}}\Big)^{1.1} \Big(\frac{T}{10^4\ \mathrm{K}}\Big)^{-1.1} \Big(\frac{\Delta V}{\mathrm{km\ s^{-1}}}\Big)^{-1} (1+Y^+)^{-1} , \qquad (15)$$

where $\nu_L$ is the frequency of the line, $T$ the plasma temperature, $\Delta V$ the FWHM of the line, and $Y^+$ the ionized helium to ionized hydrogen ratio. From the free-free continuum emission of ∼1 mJy observed at ∼20 GHz in VLA 2, assuming a wind velocity of ∼200 km s$^{-1}$, the expected peak intensity of the RRLs at these frequencies is ∼0.25 $\mu$Jy. This emission level is far below the sensitivity threshold of the spectral line observations that can be reached using existing radio interferometers from the northern hemisphere, where VLA 2 is visible. We think, however, that the detection and study of thermal RRLs in similar protostars will be highly feasible with the Square Kilometer Array (SKA) (*40*). The detection of these

lines, together with proper motion measurements, will provide unique information on the 3D kinematics of the ionized wind associated with protostars at tens of mas resolution (*40*).

Table S1. Summary of observational setups[a]

| Band/ Line | Total bandwidth (MHz) | Central frequency (GHz) | Number of channels | Channel width (kHz) | Velocity resolution (km $s^{-1}$) | Velocity coverage[b] (km $s^{-1}$) |
|---|---|---|---|---|---|---|
| Continuum observations | | | | | | |
| C[c] | 4096 | 6.0 | 2048 | 2000 | ... | ... |
| U | 6144 | 15.0 | 3072 | 2000 | ... | ... |
| K[d] | 7680 | 22.0 | 3840 | 2000 | ... | ... |
| Q | 8192 | 44.0 | 4096 | 2000 | ... | ... |
| Spectral line observations | | | | | | |
| $CH_3OH$[c] | 4 | 6.6685192 | 512 | 7.8 | 0.35 | 180 |
| $H_2O$[d] | 8 | 22.235080 | 256 | 31.3 | 0.42 | 108 |

[a]Project code is 14A-007. All observations were made using the A configuration of the VLA. Observation dates were 2014 March 15th for C, U and K bands, and 2014 April 22nd and 30th for Q band.

[b]Centered at $V_{LSR}$ = 3 km $s^{-1}$.

[c]Continuum at C band was observed simultaneously with $CH_3OH$ masers.

[d]Continuum at K band was observed simultaneously with $H_2O$ masers.

Table S2. K band continuum in VLA 2 as observed in epochs 1996 and 2014

| Epoch (yr) | Intensity Peak (mJy/beam ) | Flux Density (mJy) | Source Image Size[a] (arcsec) [p.a.°] | RMS[b] ($\mu$Jy/beam) |
|---|---|---|---|---|
| 1996 | 1.4 ± 0.2 | 1.7 ± 0.3 | 0.15 (±0.02)×0.12 (±0.01) [0±20] | 150 |
| 2014 | 0.82 ± 0.01 | 1.33 ± 0.03 | 0.171 (±0.005)×0.123 (±0.004) [65±4] | 10 |

[a]Size (FWHM) obtained from elliptical Gaussian fits to the images of VLA 2 (Fig. 2; restored circular beam = 0.12″). For epoch 1996 (data from [*10*]), VLA 2 cannot be distinguished from a point source, while for epoch 2014 (this paper) the source is clearly elongated in the northeast-southwest direction (FWHM deconvolved major axis size = 0.12″±0.01″; see also section C in this supporting online material).

[b]RMS of the images shown in Fig. 2 and from which the parameters listed in this table have been obtained.

Table S3. Parameters of the VLA 2 source at different frequencies[a]

| Frequency (GHz) | Total flux density (mJy) | Major axis size[b] (arcsec) |
| --- | --- | --- |
| | U Band | |
| 12.487 | 0.73 ± 0.02 | 0.20 ± 0.04 |
| 13.511 | 0.86 ± 0.04 | 0.20 ± 0.03 |
| 14.487 | 0.86 ± 0.04 | 0.17 ± 0.01 |
| 15.511 | 0.82 ± 0.03 | 0.15 ± 0.01 |
| 16.487 | 0.89 ± 0.04 | 0.16 ± 0.01 |
| 17.511 | 1.05 ± 0.06 | 0.16 ± 0.02 |
| | K Band | |
| 18.487 | 0.97 ± 0.03 | 0.149 ± 0.007 |
| 19.511 | 1.05 ± 0.03 | 0.154 ± 0.008 |
| 20.487 | 0.98 ± 0.03 | 0.141 ± 0.007 |
| 21.511 | 1.02 ± 0.03 | 0.133 ± 0.006 |
| 22.922 | 1.14 ± 0.03 | 0.130 ± 0.007 |
| 23.897 | 1.09 ± 0.03 | 0.118 ± 0.006 |
| 24.871 | 1.25 ± 0.05 | 0.130 ± 0.006 |
| 25.703 | 1.09 ± 0.05 | 0.103 ± 0.006 |
| | Q Band | |
| 40.487 | 1.63 ± 0.06 | ... |
| 41.151 | 1.88 ± 0.06 | ... |
| 42.249 | 2.00 ± 0.06 | ... |
| 43.511 | 2.14 ± 0.06 | ... |
| 44.487 | 2.32 ± 0.06 | ... |
| 45.511 | 2.24 ± 0.06 | ... |
| 46.487 | 2.25 ± 0.06 | ... |
| 47.447 | 2.47 ± 0.06 | ... |

[a]Parameters measured in continuum images made with 1 GHz of bandwidth. Beam sizes are in the range from ∼0.19″ (12.487 GHz) to ∼0.07″ (47.447 GHz).

[b]Deconvolved FWHM major axis size obtained from elliptical Gaussian fits. For the Q band, major axis sizes are not indicated here given that the emission at these frequencies is compact (FWHM $\lesssim$ 0.07″) and it has an important contribution (∼30%) from thermal dust continuum (see text and Fig. S4).

Table S4. Fitted parameters for different wind velocities and assuming $p = 100$

| $V_w$ $km\ s^{-1}$ | $R_0$ (mas) | $\xi$ | $t_i$ (year) |
|---|---|---|---|
| 100 | 19.29 | 9.55 | 1983.66 |
| 200 | 21.33 | 52.85 | 1984.56 |
| 300 | 21.98 | 131.33 | 1984,86 |
| 400 | 22.30 | 244.92 | 1985.02 |
| 500 | 22.48 | 393.63 | 1985.11 |
| 600 | 22.61 | 577.92 | 1985.17 |
| 700 | 22.70 | 796.93 | 1985.22 |
| 800 | 22.77 | 1051.06 | 1985.25 |
| 900 | 22.81 | 1340.29 | 1985.28 |
| 1000 | 22.85 | 1665.46 | 1985.30 |

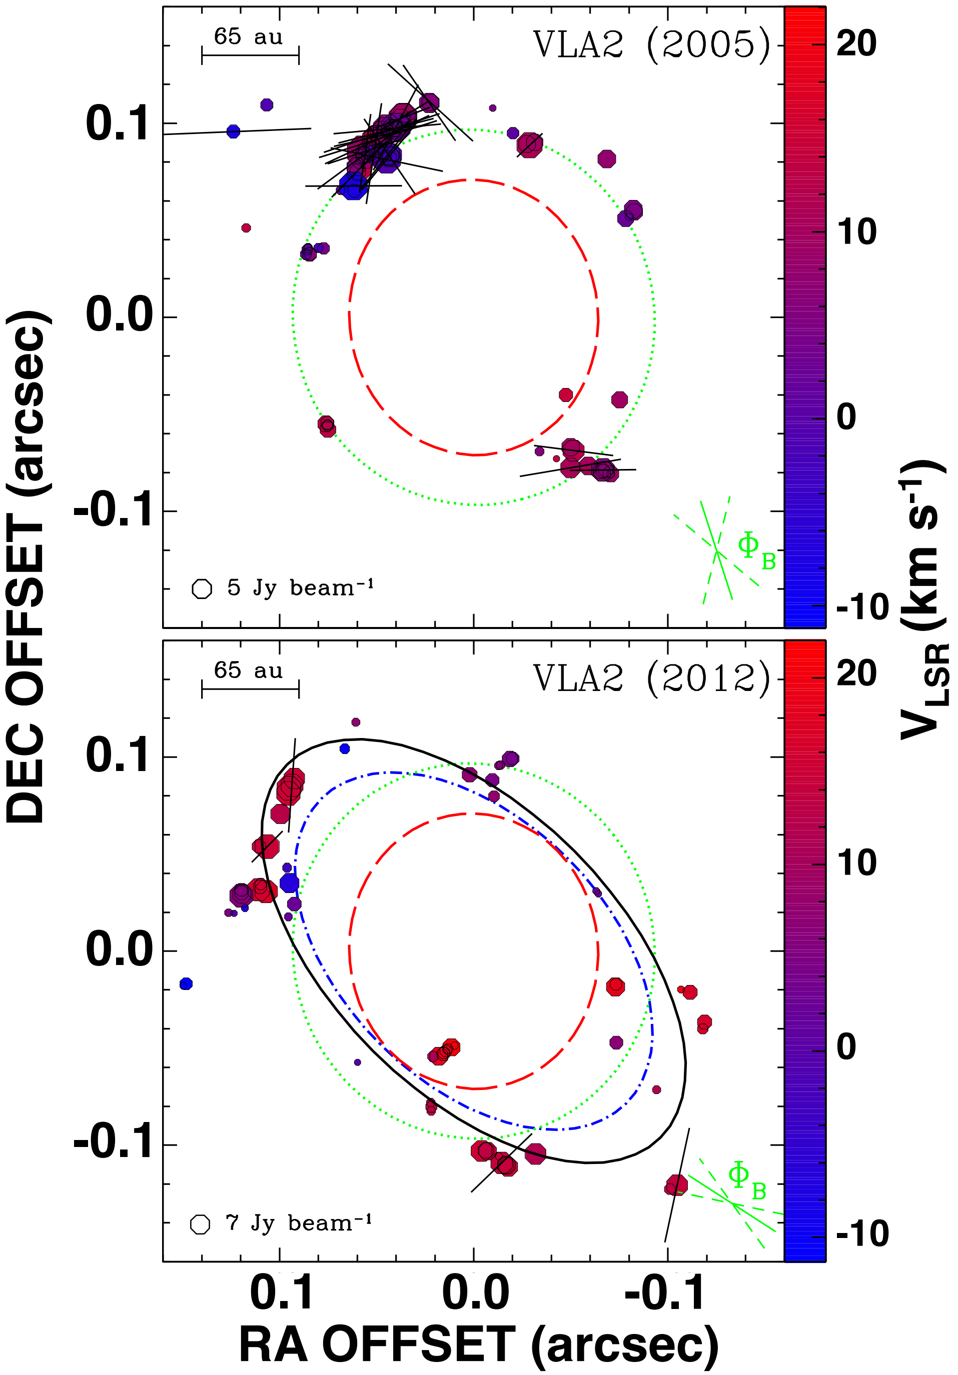


Fig. S1.— Evolution of the water maser shell and magnetic field around VLA 2 from epoch 2005 (top panel) to 2012 (bottom panel) as observed by (*14*) with VLBI. The color scale indicates the LSR radial velocity of the masers (octagonal symbols, scaled logarithmically according to their flux densities). Linear polarization vectors of the masers are also indicated. The error-weighted orientation of the magnetic field ($\Phi_B$) as derived from the polarization of the masers is indicated in the bottom-right corners of the two panels. A comparison of the elliptical fits of the water maser distribution observed in the past 13 years is also shown: red dashed ellipse (epoch 1999), green dotted ellipse (epoch 2005), blue dot-dashed ellipse (epoch 2007), black solid ellipse (epoch 2012). The water maser shell has evolved from an almost circular shell (∼185 au diameter; epoch 1999) to an elliptical structure (∼354×190 au) oriented northeast-southwest (epoch 2012). The magnetic field changed also its orientation, following the direction of the water maser elliptical shell. [Figure adapted from (*14*)].

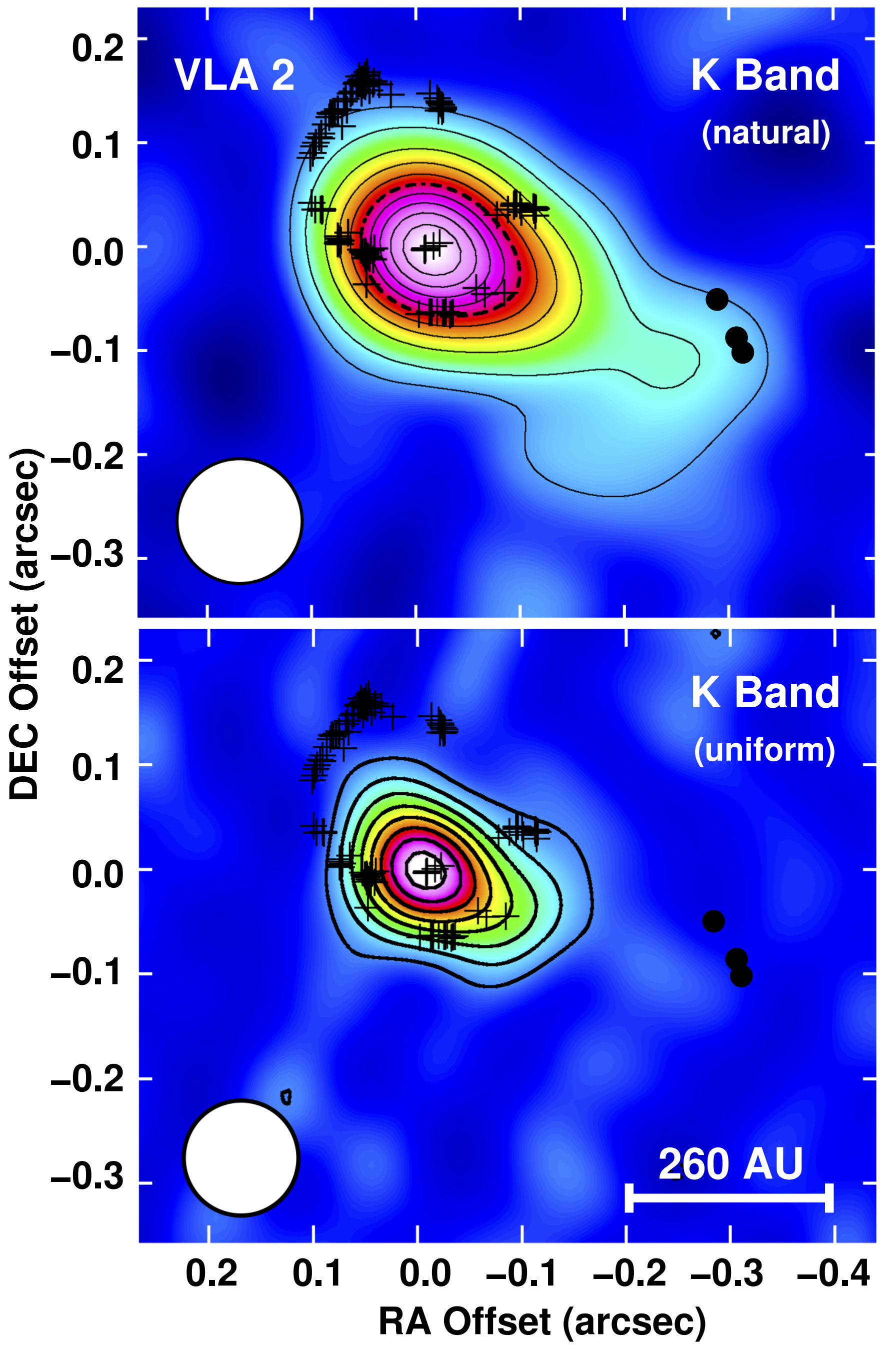


Fig. S2.— K band continuum emission of VLA 2 observed in 2014 and imaged with natural (top panel) and uniform (bottom panel) weighting of visibilities. Contours are 5, 10, 20, 30, 40, 50, 60, 70, 80, and 90% the peak intensity (0.82 mJy beam$^{-1}$) (top panel, rms = 10 $\mu$Jy beam$^{-1}$; this figure is the same as the one shown in Fig. 2, where the contour level of the 50% of the peak emission is shown with dashed line), and -3, 3, 6, 9, 12, 15, 18, 21, 24 × 30 $\mu$Jy beam$^{-1}$ (the rms of the uniform image, bottom panel). The water (plus symbols) and methanol (black dots) maser positions as observed with the VLA in 2014 (this work) are also indicated. The elongation of the core of the radio continuum emission of VLA 2 is also clearly seen in the image with uniform weight. The beam sizes are shown in the bottom left corner of each panel.

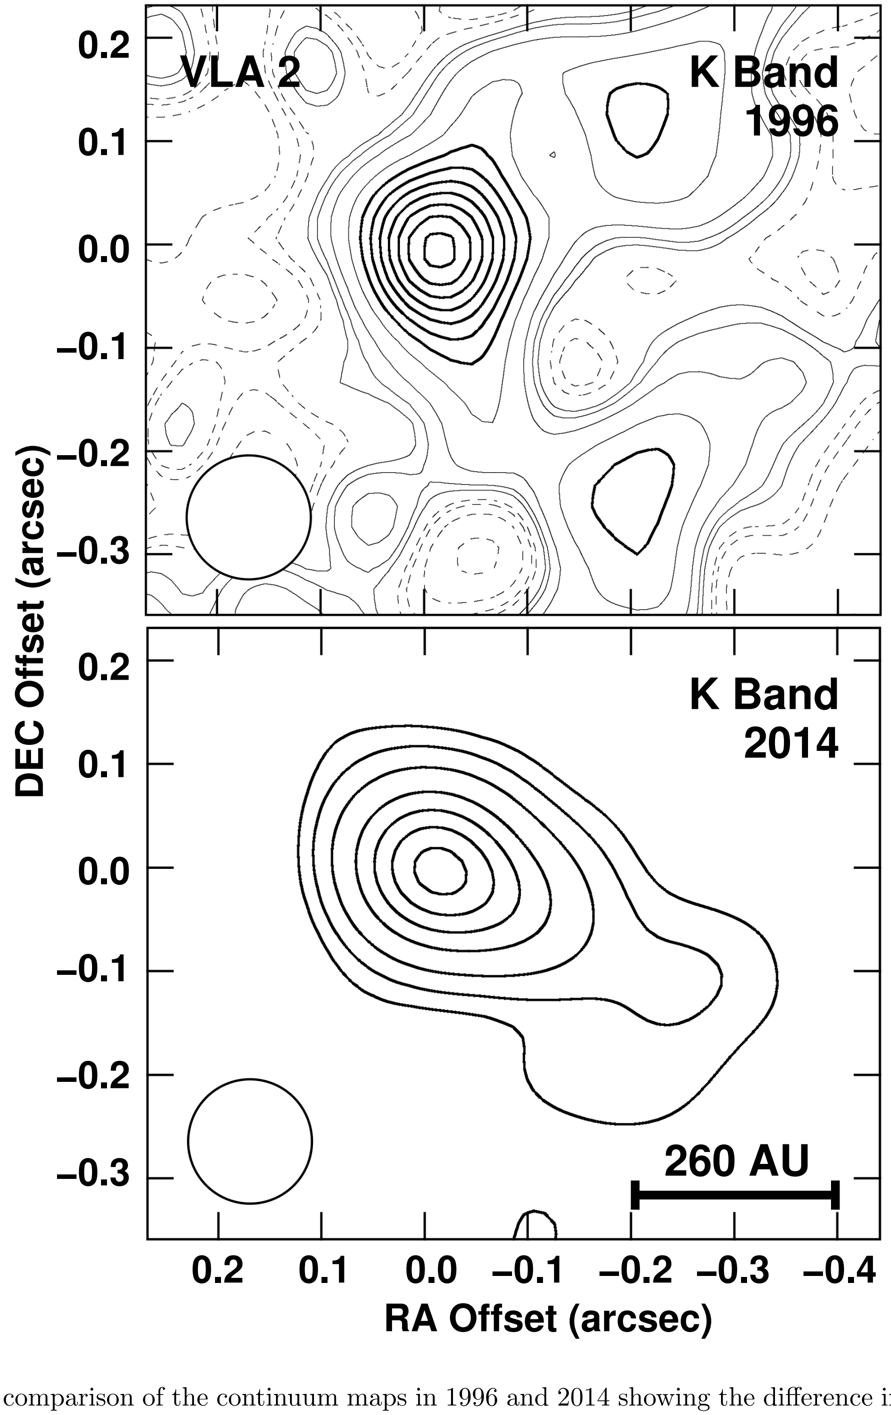


Fig. S3.— A comparison of the continuum maps in 1996 and 2014 showing the difference in the sensitivity between epochs. In both panels, contours are −2, −1, −0.5, −0.25, 0.25, 0.5, 1, 2, 3, 4, 5, 6, 7, 8, 9, and 10 times 150 $\mu$Jy beam$^{-1}$, the rms noise of the 1996 map. Thick contours are over 3 times while thin contours are below. Thin dashed contours are negative.

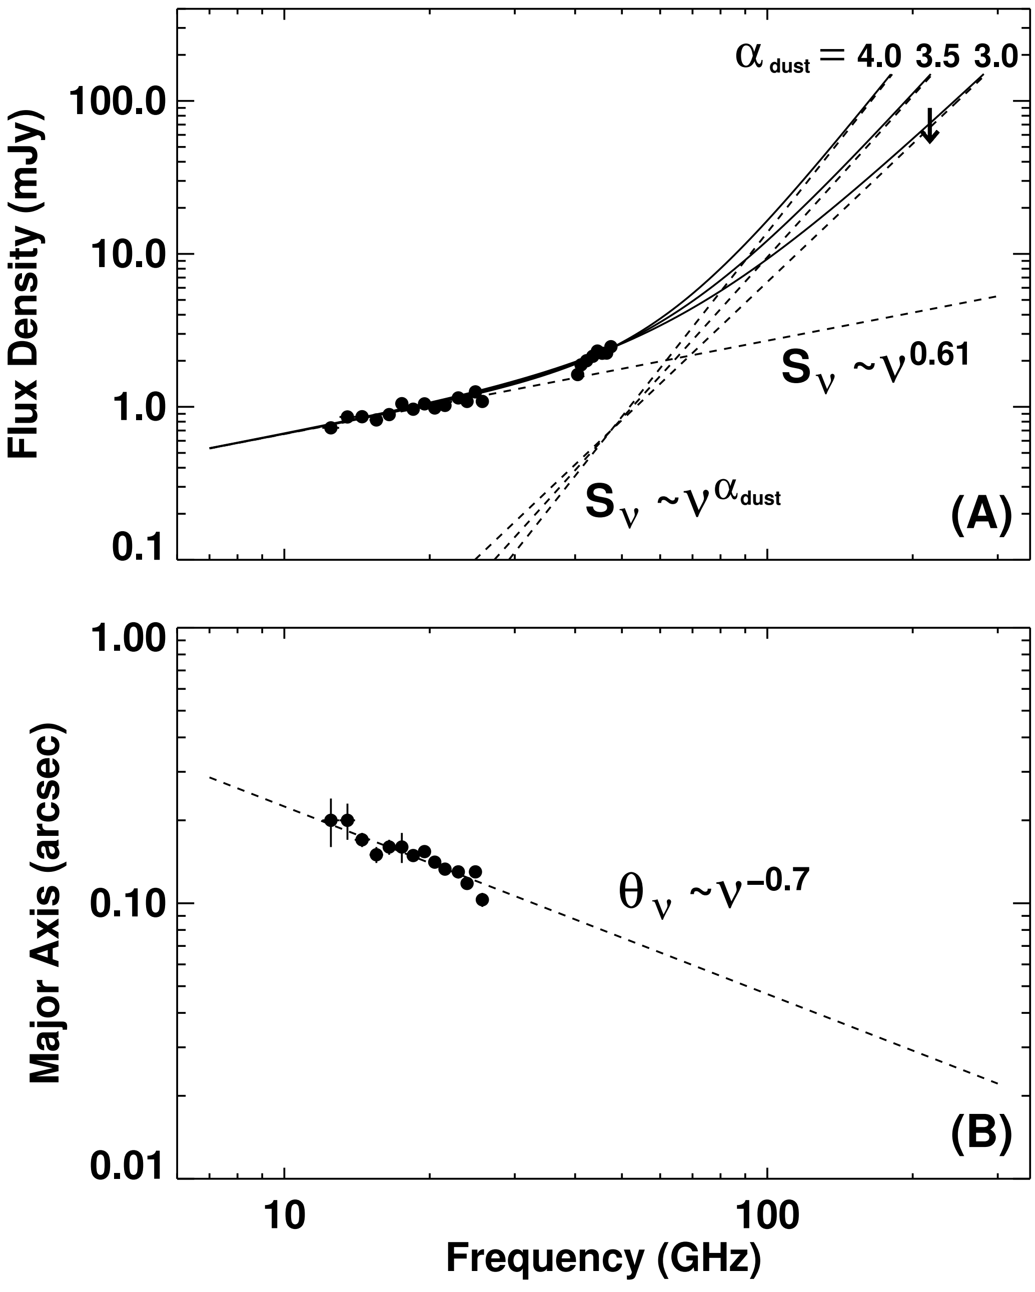


Fig. S4.— **(A)** Spectral energy distribution of VLA 2 at U, K, and Q bands. While the emission at the lowest frequencies is dominated by free-free emission with a spectral index $\alpha \simeq 0.61 \pm 0.04$ ($S_\nu \propto \nu^\alpha$), at the highest frequencies, the emission deviates from this behavior (~30%, ~0.5 mJy), showing a steeper spectral index that can be explained with the contribution of thermal dust emission with spectral index $\alpha_{dust}$. Three different contributions of dust emission corresponding to values $\alpha_{dust}$ = 3.0, 3.5, and 4.0 are shown. The solid lines are the sum of both contributions (free-free + dust continuum). The upper limit to the flux density at 217 GHz is from the SMA observations of (*20*). **(B)** Plot showing the decrease of the size of the major axis of the free-free emission of VLA 2 as function of frequency (U and K bands). The size ($\theta$) can be fitted as a power-law in the form $\theta \propto \nu^\beta$, with $\beta \simeq -0.7 \pm 0.1$. This behavior for the flux density and the size of the major axis as function of frequency, is in good agreement with the one expected for a thermal, collimated ionized wind driven by a protostar (see text).
